# Supplementary material for: From Optimal Transport to Efficient Mechanisms for the $m$-Capacitated Facilities Location Problem with Bayesian Agent
Source: arXiv:2312.16034 source file (2024-06-15)
Supplement: Supplementary file 1 [file appendix.tex]

\appendix
